# Supplementary material for: Convolutional Prompting meets Language Models for Continual Learning
Source: arXiv:2403.20317 source file (2024-03-29)
Supplement: Supplementary file 2 [file preamble.tex]

%
% --- inline annotations
%
% \usepackage[dvipsnames]{xcolor}
%%%%%%% for todos%%%%%%%%%%%%%%%%%%%%%%%%%%%%%%%%
\usepackage{color}
\definecolor{forest-green}{rgb}{0.59, 0.82, 0.47}
\definecolor{grey}{rgb}{0.93, 0.93, 0.93}
\definecolor{new-blue}{rgb}{0.5, 0.5, 0.99}
\definecolor{peach}{rgb}{0.99, 0.89, }
\definecolor{darkorchid}{rgb}{0.6, 0.2, 0.8}
\newcommand{\todo}[1]{\textcolor{red}{TODO: #1}}
\newcommand{\sg}[1]{\textcolor{cyan}{[SG: #1]}}
\newcommand{\anurag}[1]{\textcolor{blue}{#1}} % Anurag: 
\newcommand{\vinay}[1]{\textcolor{magenta}{Vinay: #1}}
\newcommand{\doubt}[1]{\textcolor{red}{DOUBT: #1}}
\newcommand{\abir}[1]{{\textcolor{darkorchid}{[AD: #1]}}}
\newcommand{\riddhiman}[1]{\textcolor{forest-green}{[Riddhiman: #1]}}
\usepackage{soul}
\newcommand{\anust}[1]{\textcolor{blue}{\st{ #1}}}
\newcommand{\model}{\texttt{ConvPrompt}}
%%%%%%%%%%%%%%%%%%%%%%%%%%%%%%%%%%%%%%%%%%%%%%%%
% --- disable by uncommenting  
% \renewcommand{\TODO}[1]{}
% \renewcommand{\todo}[1]{#1}
